# Supplementary material for: Safety-Aware Preference-Based Learning for Safety-Critical Control
Source: arXiv:2112.08516 source file (2022-04-11)
Supplement: Supplementary file 1 [file lemmaProof.tex]

\label{apdx:lemma_proof}

In this appendix we present the proof of Lemma \ref{lem:safety_reduced_model} which establishes the input-to-state safety of $\mathcal{S}$. Recall that Lemma \ref{lem:safety_reduced_model} is given as: 

\begin{lemma*} 
\textit{
Consider system~(\ref{eq:full_system}), velocity $\mb{v}$ satisfying~(\ref{eq:desired_velocity_ISSf}), tracking error $\bs{\eta}$ given by~(\ref{eq:tracking_error}), and a tracking controller $\mb{u}=\Theta(\mb{x},\bs{\xi})$ satisfying Assumption \ref{assp:ISS-tracking}.
Then, $\mathcal{S}$ as defined in \eqref{eq:safe_set_ro} is ISSf, associated with the following forward invariant set:
\begin{equation}
    \mathcal{S}_{\bs{\eta}} = \left\{ (\mb{x},\bs{\xi}) \in \R^n \times \R^k : h_R(\mb{x}, \bs{\rho}) \geq  - \frac{1}{4ab}\overline{\eta}^2 \right\}.
    % \label{eq:invariant_set}
\end{equation}
} 
\end{lemma*}
\noindent
\begin{proof}
\begin{align}
    \dot{h}_R(\mb{x}, \rho) & = \frac{\partial h }{\partial \mb{x}}(\mb{f}(\mb{x}) + \mb{g}(\mb{x})(\mb{v}_d + \eta))  \\
    & \geq -a h(\mb{x}, \rho) + b \left\Vert \frac{\partial h_R}{\partial \mb{x}}\mb{g}(\mb{x})  \right\Vert^2 - \left\Vert \frac{\partial h_R}{\partial \mb{x}}\mb{g}(\mb{x}) \right\Vert \left \Vert \eta \right\Vert\\
    & \geq - ah_R(\mb{x}, \rho) +   \left(\sqrt{b}\Vert \frac{\partial h_R}{\partial \mb{x}} \mb{g}(\mb{x}) \Vert - \frac{1}{2 \sqrt{b} } \Vert \eta \Vert \right)^2 - \frac{1}{4b}\Vert \eta \Vert^2 \\
    & \geq - a h(\mb{x}, \rho) - \frac{1}{4b} \overline{\eta}^2. 
\end{align}
So 
\begin{equation}
    h(\mb{x}, \rho)+ \frac{1}{4ab}\overline{\eta}^2 \leq 0 \implies \dot{h}_R \geq 0 
\end{equation}
which also implies that $\frac{d}{dt}(h_R + \frac{1}{4ab}\Vert \overline{\eta} \Vert^2) \geq 0 $ for all $h(\mb{x}, \rho) + \frac{1}{4ab}\Vert \overline{\eta}\Vert^2 = 0 $, so the set $\mathcal{S}_{e,\mb{d}}$ is invariant with the class $\mathcal{K}$ function $\iota(\overline\eta) = \frac{1}{4ab}\overline{\eta}^2$ by Nagumo's theorem \cite{nagumo1942lage} and thus the set $\mathcal{S}$ is ISSf by defition. 
\end{proof}
