# Supplementary material for: Safety-Aware Preference-Based Learning for Safety-Critical Control
Source: arXiv:2112.08516 source file (2022-04-11)
Supplement: Supplementary file 2 [file pblAppdx.tex]

We model the posterior as proportional to the product of likelihood and the prior:
\begin{align*}
    \P(\util \mid \data) \propto \P(\data \mid \util)\P(\util),
\end{align*}
where we define the Gaussian prior over $\util$ as:
\begin{align*}
    \P(\util) = \frac{1}{(2\pi)^{\frac{|\act|}{2}} | \Sigma^{\textrm{pr}}| ^{\frac{1}{2}}} \exp \left( -\frac{1}{2}\util^{T}(\Sigma^{\textrm{pr}})^{-1} \util \right),
\end{align*}
with $\Sigma^{\textrm{pr}} \in \R^{|\act| \times |\act|}$ being a prior covariance matrix with each element $[\Sigma^{\textrm{pr}}_{ij}] = \mathcal{K}(\act_i,\act_j)$ and any kernel $\mathcal{K}$. In this work, we use a squared exponential kernel:
\begin{align*}
    \mathcal{K}_{\text{SE}}(\act,\act') = \sigma^2 \exp\left( - \frac{(\act - \act')^2}{2\mb{l}^2} \right) + \varepsilon,
\end{align*} 
where $\sigma \in \R$ is the output variance hyperparameter, $\mb{l} \in \R^d$ is a vector of lengthscales for each dimension of $\act$, and $\varepsilon$ is a kernel noise hyperparameter. The output variance $\sigma$ dictates the expected amplitude of the underlying function. The lengthscales $l_i$, $i \in \{1,\dots,d\}$, are hyperparameters that dictate the expected maximum amount that the underlying function varies in each dimension (the ``wiggliness'').

% \section{Andrew's Dynamics}
% \textcolor{red}{
% Consider the following nonlinear control-affine cascaded system:
% \begin{align}
%     \dot{\mb{x}} &= \mb{f}(\mb{x})+\mb{g}(\mb{x})\bs{\kappa}(\bs{\xi}) \\ \dot{\bs{\xi}} &= \mb{f}_{\bs{\xi}}(\mb{x},\bs{\xi}) + \mb{g}_{\bs{\xi}}(\mb{x},\bs{\xi})\mb{u}
% \end{align}
% with states $\mb{x},\bs{\xi}\in\R^n$, input $\mb{u}\in\R^m$, and functions $\mb{f}:\R^n\to\R^n$, $\mb{g}:\R^n\to\R^{n\times n}$, $\mb{f}_{\bs{\xi}}:\R^n\times\R^n\to\R^n$, and  $\mb{g}_{\bs{\xi}}:\R^n\times\R^n\to\R^{n\times m}$ assumed to be locally Lipschitz continuous on their domains. These dynamics may represent systems described by the Euler-Lagrange equations, such as robotic systems, where $\mb{x}$ and $\bs{\xi}$ reflect the position and velocity coordinates, respectively, and the input $\mb{u}$ reflects forces and torques applied to the system. 
% Motivated by \cite{molnar2021model}, this cascaded model is taken for two reasons.
% The first reason is that the dynamics of the state $\bs{\xi}$ may often be very complicated, such as in the case of legged locomotion \AT{CITE}.
% It is often the case that the control of these dynamics is treated as a separate subsystem, 
% The second reason is that many safety requirements (such as collision-avoidance) are specified as constraints on the position, or the state $\mb{x}$, rather than on both states $\mb{x}$ and $\bs{\xi}$. 
% There exists $\mb{k}:\R^{n?}\to\R^m$ such that:
% \begin{equation}
%     \Vert \bs{\xi}-\bs{\xi}_d(t)\Vert \leq \epsilon
% \end{equation}
% }
